# Supplementary material for: Information-theoretical measures identify accurate low-resolution representations of protein configurational space
Source: arXiv:2205.08437 ancillary file (2022-05-17)
Supplement: Supplementary file 1 [file supp.pdf]

Supporting Material for

# *Information-theoretical measures identify accurate low-resolution representations of protein configurational space*

Margherita Mele,[a] Roberto Covino,[b] and Raffaello Potestio[a,c,*]

[a] *Physics Department, University of Trento, via Sommarive, 14 I-38123 Trento, Italy*
[b] *Frankfurt Institute for Advanced Studies, 60438 Frankfurt am Main, Germany*
[c] *INFN-TIFPA, Trento Institute for Fundamental Physics and Applications, I-38123 Trento, Italy*

This document consists of two parts. In the first, we report the results obtained in the application of the Relevance and Resolution framework on the database composed of 12 proteins. In particular, for each biological system considered we show the relevance and resolution curves plotted by 7 clustering algorithms, varying the number of clusters, on three selections of atoms (all, $C_\alpha$, and $C_\beta$ atoms). In the second, the results obtained in the study of the humanised IgG4 monoclonal antibody are reported. In this section the plot showing the distribution of points in the 2D diffusion space resulting from the HR representation and some LR ones are compared.

## 1 Exploratory Analysis

The series of figures (Fig.1, Fig.2 and Fig.3) shows the relevance-resolution curves obtained by applying 7 clustering algorithms on the MD trajectory pertaining to 12 biological systems described at three levels of detail (all atom, $C_\alpha$ atoms, and $C_\beta$ atoms). A visual inspection of these plots shows a systematic behaviour in the curves drown by a given clustering algorithm, regardless of the biological system. This systematic pattern is confirmed if we look at the behaviour of the MSR values ($\overline{MSR}$), the area under the relevance and resolution curves normalised with respect to the value obtained from random clustering (Fig.4). The Fig.4 clearly shows that not all algorithms perform in the same way. There are algorithms whose associated curves, and MSR values, are always above the random curve regardless of the system and selection used, and others whose performance depends on the system's representation. Given its properties, MSR proves to be a useful quantity for rating the performance of a clustering method in identifying reduced but informative partitions. For a more in-depth analysis of these properties and an explanation of how to employ them, see the main text of this paper.

$*$ raffaello.potestio@unitn.it

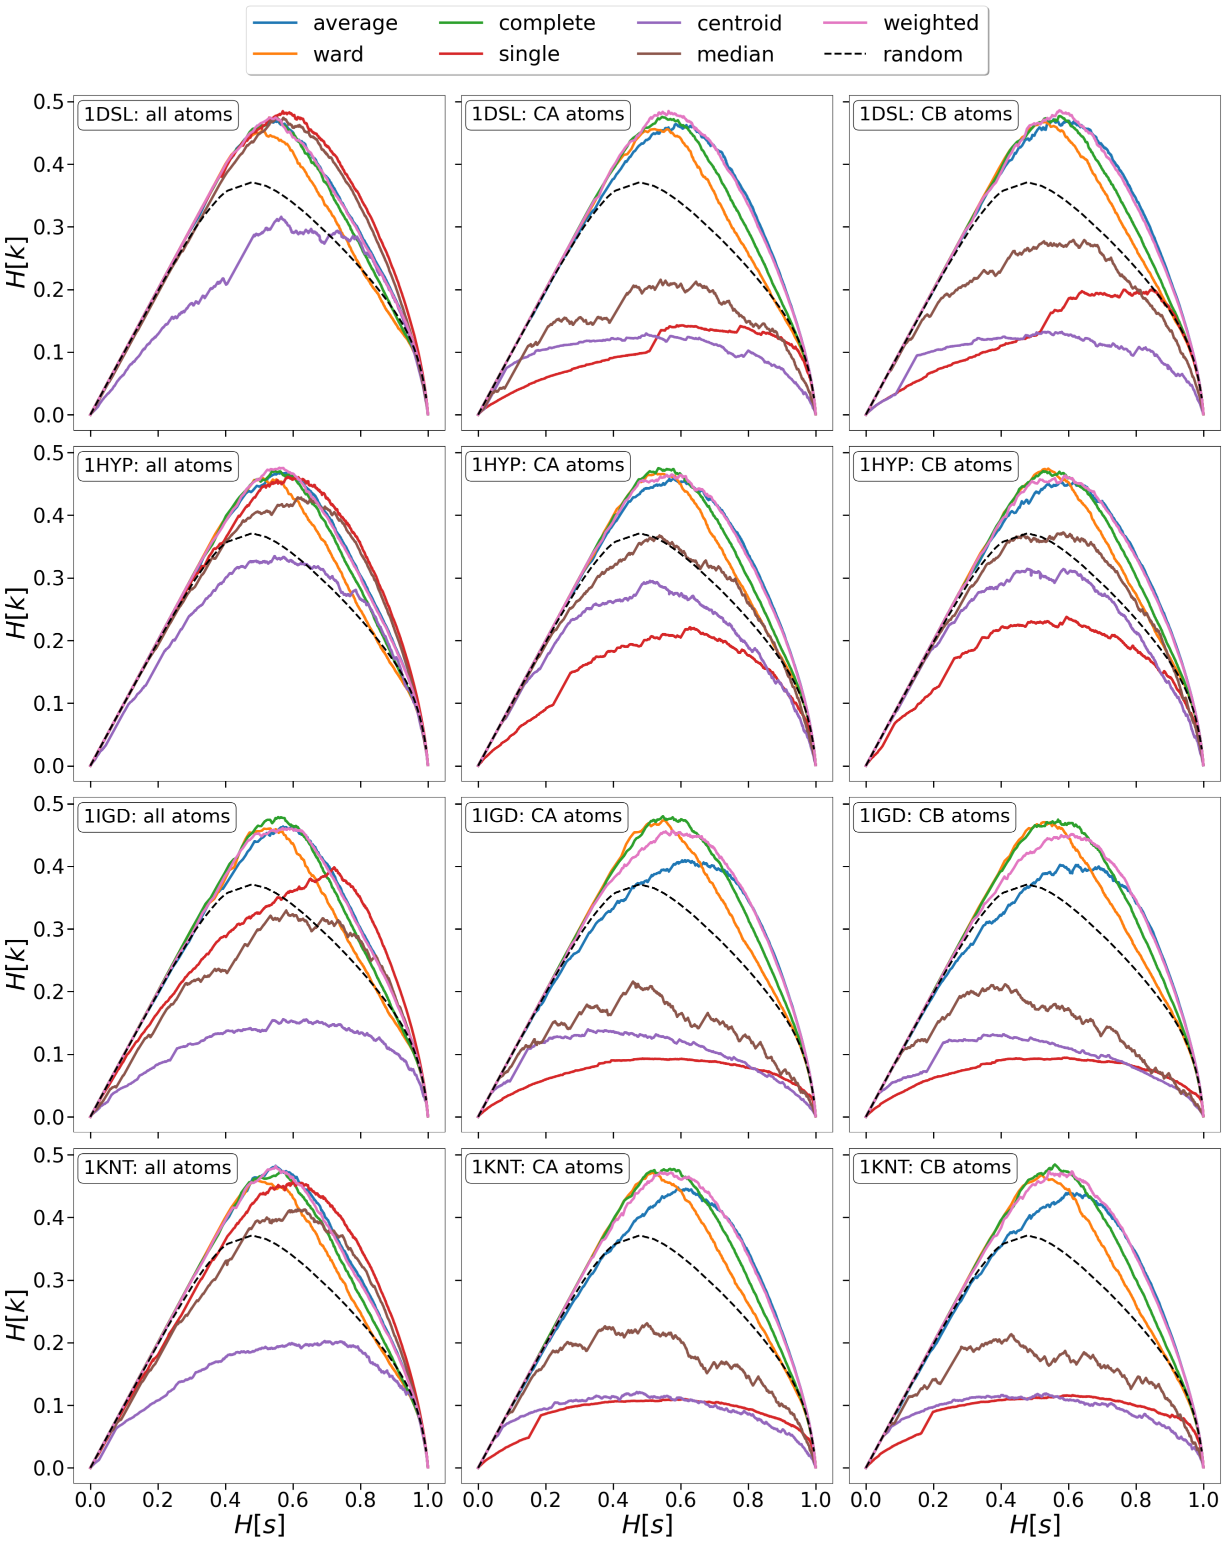


Figure 1: Each image in this series of graphs shows relevance and resolution curves obtained by clustering a MD trajectory varying the number of clusters from 1 up to the total number of frame. The curves, in each plot, differ for the protocol adopted in the clustering procedure as defined in the legend. Each row in the figure reports the results obtained for a biological system analysed exploring three atomic selection: *all atoms* (on the left), $C_\alpha$ *atoms*(in the middle) and $C_\beta$ *atoms* (on the right). The biological system reported in this panel (from top to bottom) are defined by the PDB code: 1DSL, 1HYP, 1IGD, 1KNT.

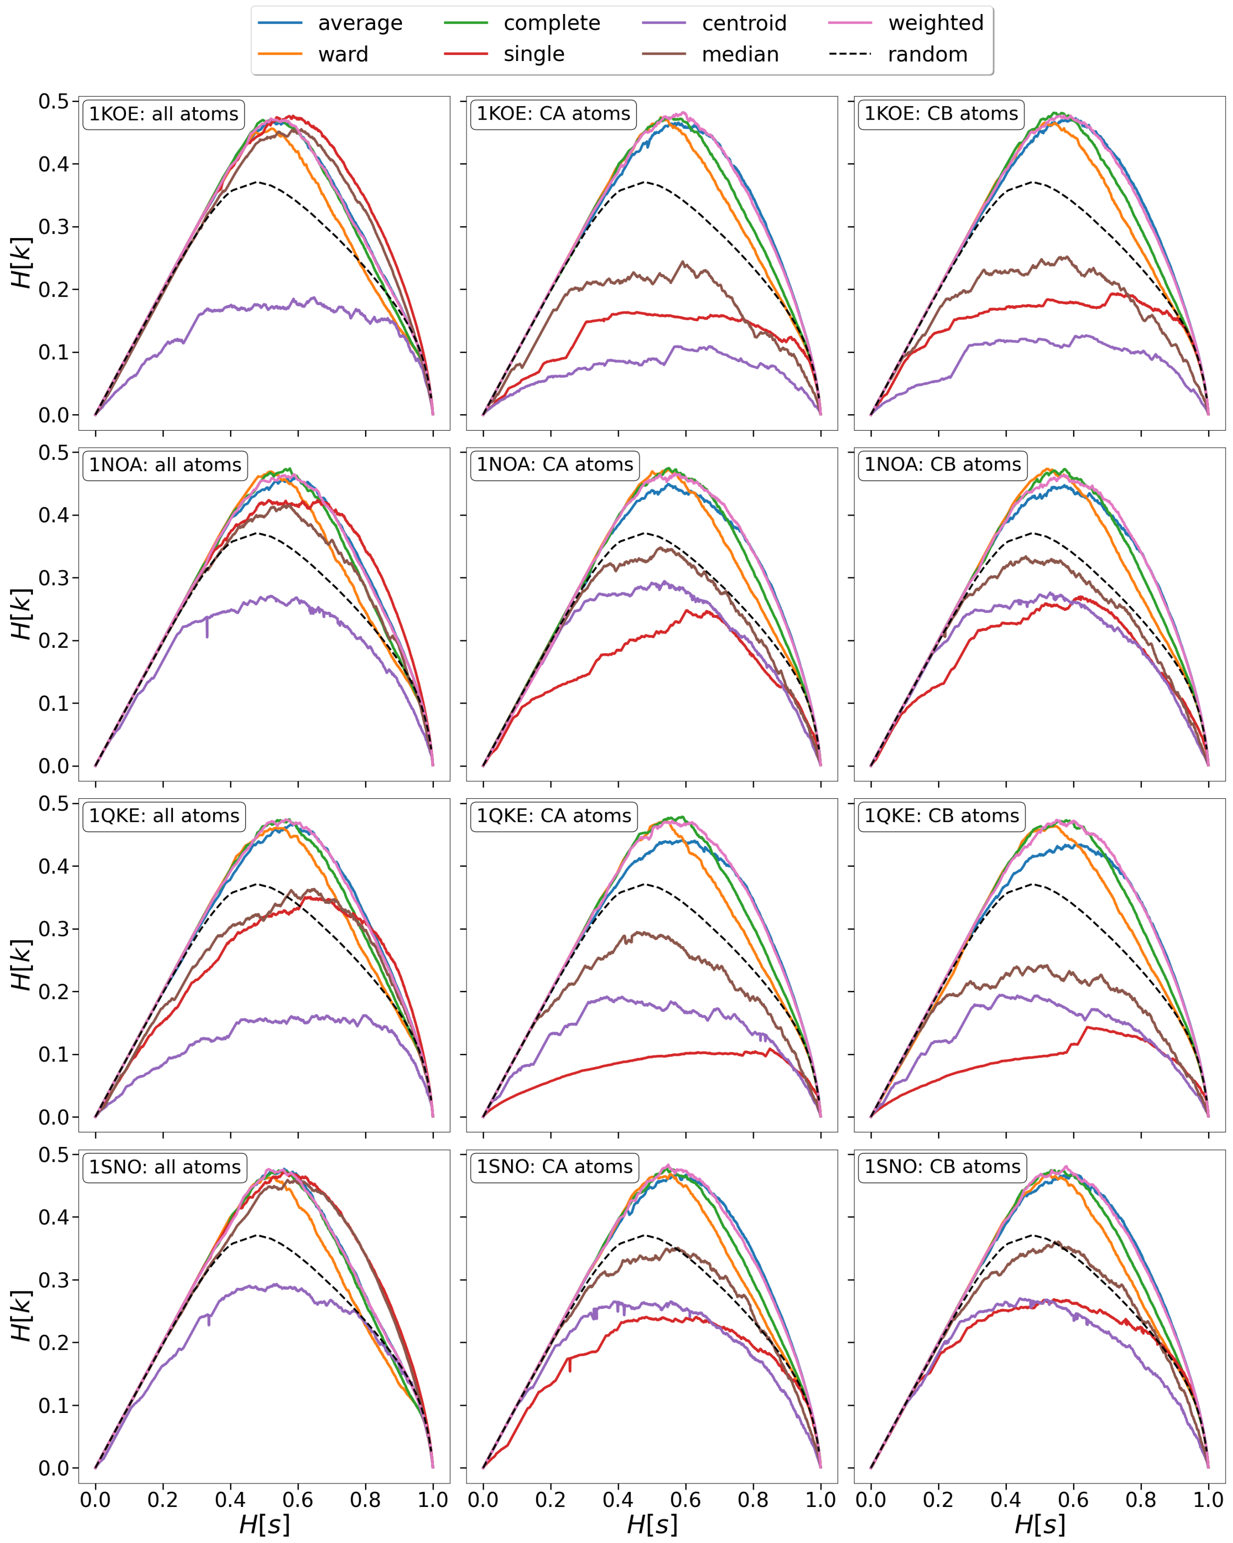


Figure 2: Each image in this series of graphs shows relevance and resolution curves obtained by clustering a MD trajectory varying the number of clusters from 1 up to the total number of frame. The curves, in each plot, differ for the protocol adopted in the clustering procedure as defined in the legend. Each row in the figure reports the results obtained for a biological system analysed exploring three atomic selection: *all atoms* (on the left), $C_\alpha$ *atoms*(in the middle) and $C_\beta$ *atoms* (on the right). The biological system reported in this panel (from top to bottom) are defined by the PDB code: 1KOE, 1NOA, 1QKE, 1SNO.

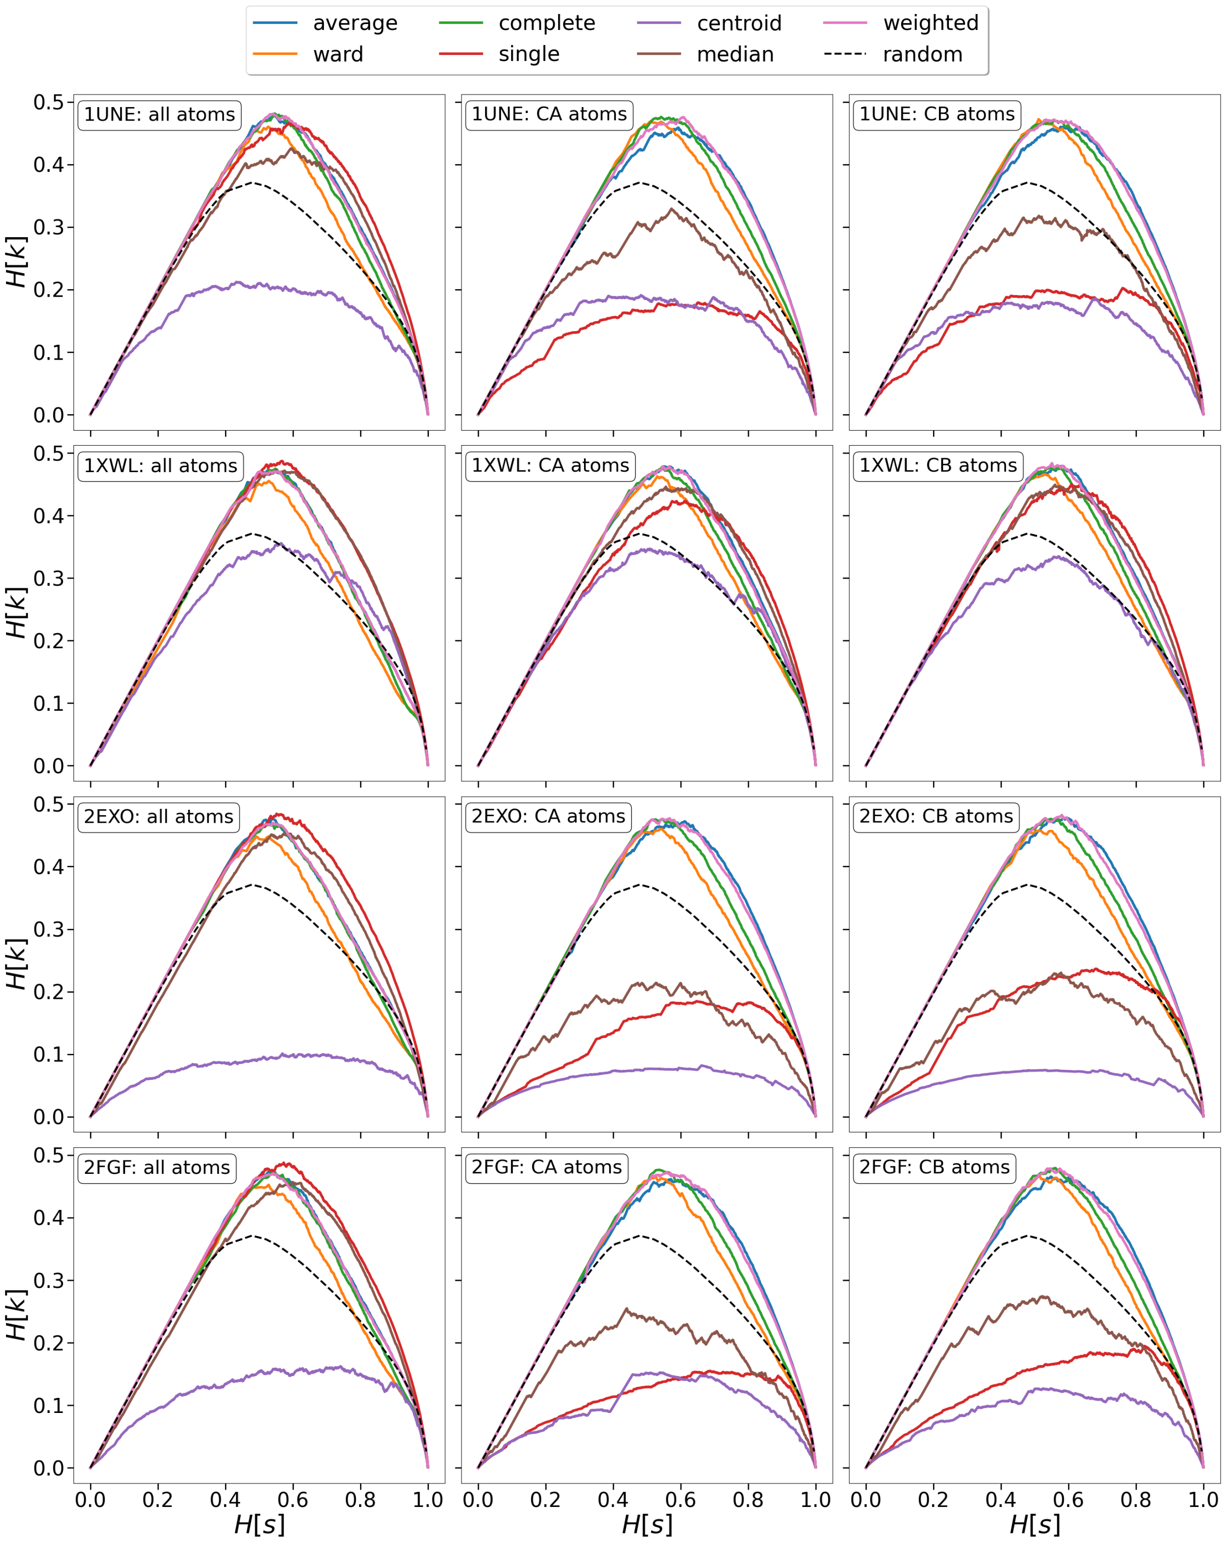


Figure 3: Each image in this series of graphs shows relevance and resolution curves obtained by clustering a MD trajectory varying the number of clusters from 1 up to the total number of frame. The curves, in each plot, differ for the protocol adopted in the clustering procedure as defined in the legend. Each row in the figure reports the results obtained for a biological system analysed exploring three atomic selection: *all atoms* (on the left), $C_\alpha$ *atoms*(in the middle) and $C_\beta$ *atoms* (on the right). The biological system reported in this panel (from top to bottom) are defined by the PDB code: 1UNE, 1XWL, 2EXO, 2FGF.

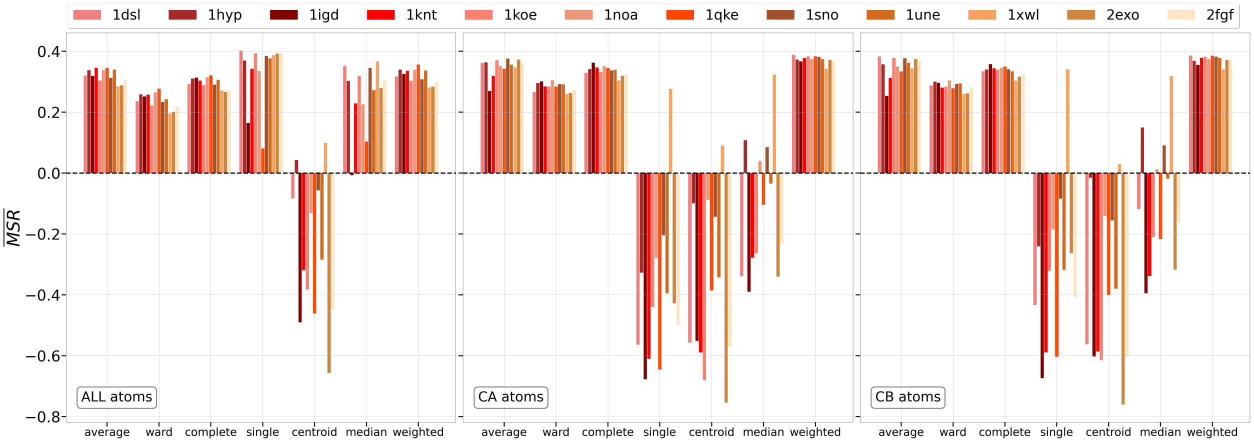


Figure 4: The figure shows the values of normalized MSR (the area under the RR-curves) against the clustering algorithm used to generate the curve. The colours identify the biological system on which the analysis was carried out as shown in the legend. The three graphs differ in the selection of atoms on which the RMSD matrix used for clustering was calculated: *all atoms* on the left , $C_\alpha$ *atoms* in the middle and $C_\beta$ *atoms* on the right.

## 2 Humanised IgG4 monoclonal antibody

In this section we show that the relevance and resolution framework is robust also in the case of biological systems of larger size and greater dynamical variability than the adenylate kinase, such as the humanised IgG4 monoclonal antibody. This comparison is performed, as with adenylate kinase, by comparing the distribution of points, frames or clusters, in the 2D diffusion space. We compare here the representations obtained through three clustering protocols (average, complete and single linkage) for three number of clusters $K = 311$, $K = 351$ and $K = 901$. From Fig.5, Fig.6 and Fig.7 it can be seen that there is an optimal correspondence between the high-resolution (HR) and low-resolution (LR) spaces for partitions given by average and complete methods. In these cases, as the number of clusters increases, more and more details of the HR space are brought into the LR one. However, concerning the single method, it can be seen that frames which are very far apart in HR space are all mapped to the same clusters, thus producing a less significant partitioning of the system. In some cases it fails to reproduce any detail of the HR space at all (Fig.5). In addition, as the number of clusters increases, these clusters are arranged in regions that are already sufficiently sampled and therefore do not contribute much information to the representation. What has just been shown, demonstrates that the RR-framework is able to identify meaningful reduced representations even in case of structurally and biologically complex systems such as an antibody.

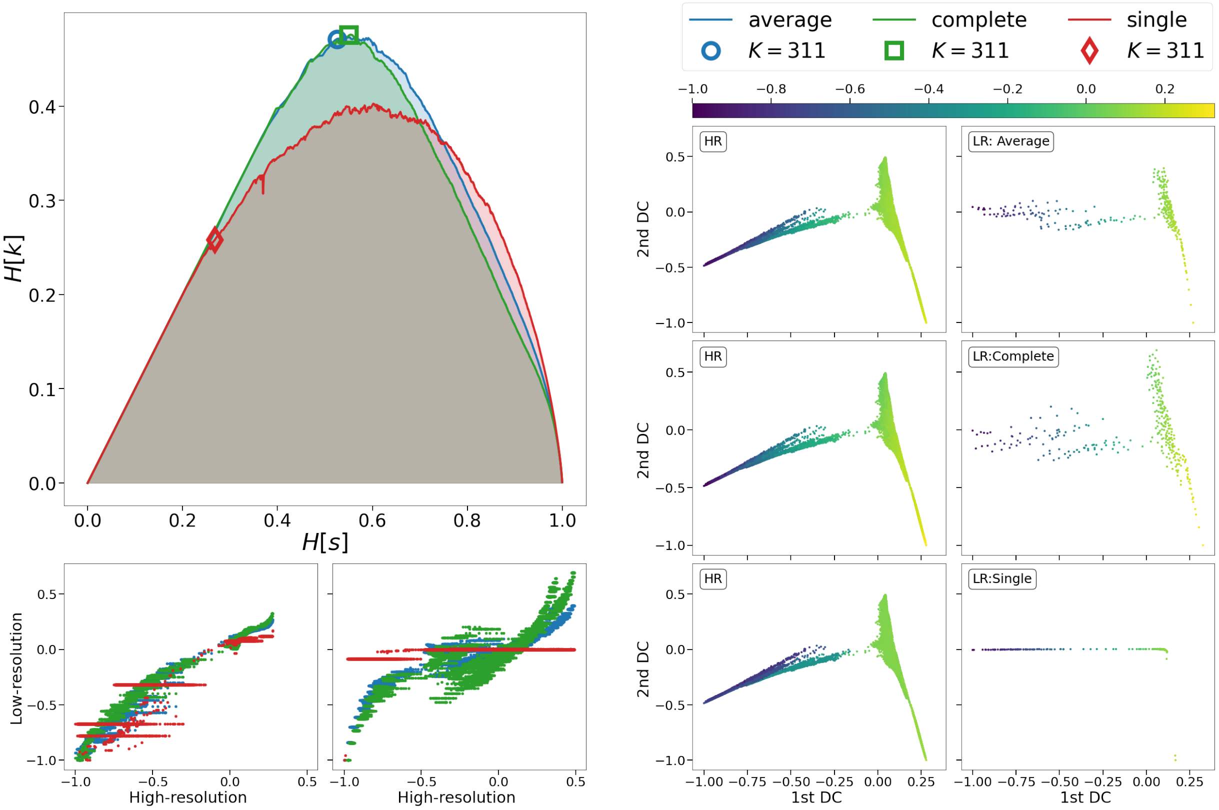


Figure 5: The panel aims to quantitatively and qualitatively compare the low-resolution representation (LR) of the configurational space explored by the humanised IgG4 monoclonal antibody during an MD simulation. These representations are obtained through three clustering protocol, for a number of clusters $K = 311$. The upper left-hand side of the figure shows the relevance-resolution curves obtained from clustering the MD trajectory, according to the average-linkage (blue), complete-linkage (green) and single-linkage (red) protocols. The system was analysed using a coarse representation in which only $C_\beta$ *atoms* are considered. The markers show where on the respective curve the low-resolution representations obtained by partitioning the system into a $K = 311$ clusters lie. On the right-hand side the graphs representing the points projected onto the space spanned by the first two diffusion coordinates. The graphs on the left show the diffusion space resulting from high-resolution representation (HR) where each point is a frame of the MD simulation and the distance between them is given by the RMSD calculated on the $C_\beta$ atoms. On the right the two-dimensional diffusion space resulting from the LR representation where each point is the centroid of a cluster and the distance between points is the linkage measure that produced the partition (average-linkage on top, complete-linkage in the middle and single-linkage on bottom). In both high and low resolution space, the points are coloured with respect to the value taken by the first diffusion coordinate in the low-resolution space. The lower right corner of the figure shows the scatter plot in which the first and second diffusion coordinates (DC) of the high-resolution space are plotted against the corresponding coordinate of the low-resolution space.

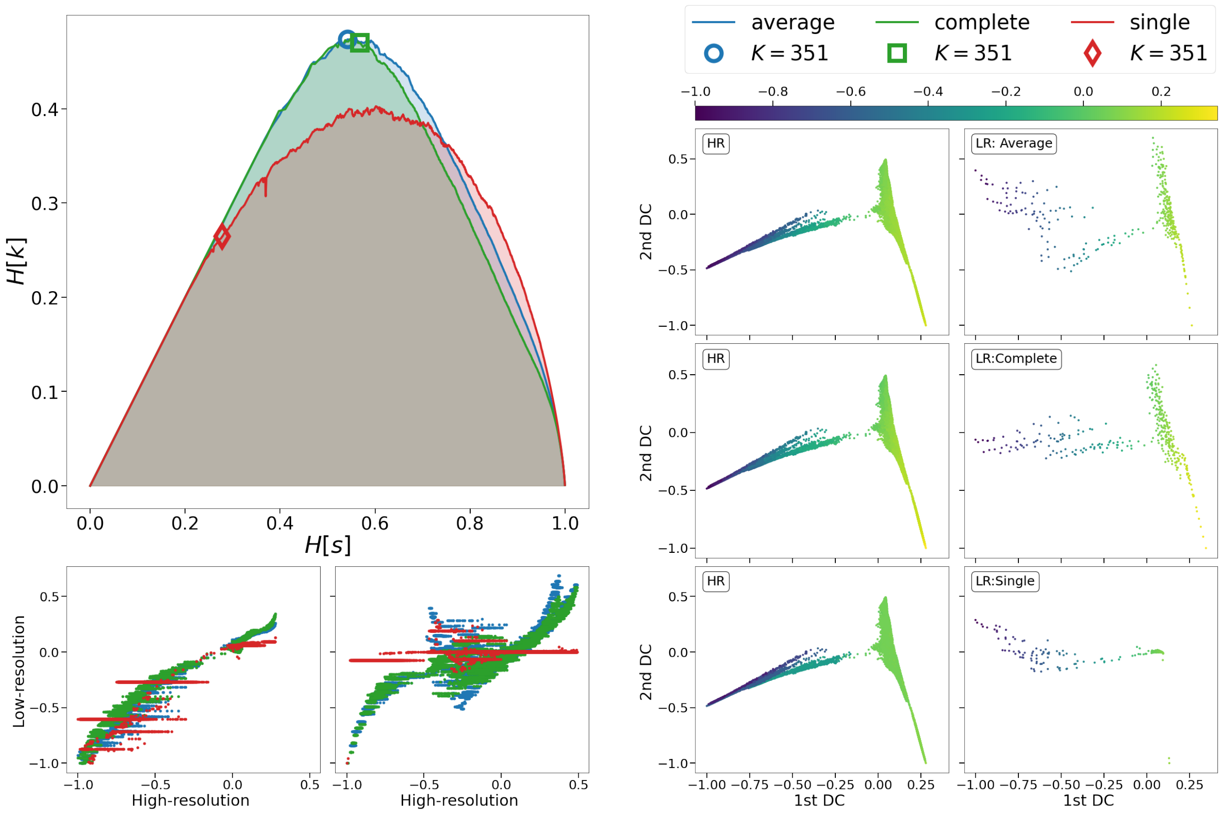


Figure 6: The panel aims to quantitatively and qualitatively compare the low-resolution representation (LR) of the configurational space explored by the humanised IgG4 monoclonal antibody during an MD simulation. These representations are obtained through three clustering protocol, for a number of clusters $K = 351$. The upper left-hand side of the figure shows the relevance-resolution curves obtained from clustering the MD trajectory, according to the average-linkage (blue), complete-linkage (green) and single-linkage (red) protocols. The system was analysed using a coarse representation in which only $C_\beta$ *atoms* are considered. The markers show where on the respective curve the low-resolution representations obtained by partitioning the system into a $K = 351$ clusters lie. On the right-hand side the graphs representing the points projected onto the space spanned by the first two diffusion coordinates. The graphs on the left show the diffusion space resulting from high-resolution representation (HR) where each point is a frame of the MD simulation and the distance between them is given by the RMSD calculated on the $\mathrm{C}_\beta$ atoms. On the right the two-dimensional diffusion space resulting from the LR representation where each point is the centroid of a cluster and the distance between points is the linkage measure that produced the partition (average-linkage on top, complete-linkage in the middle and single-linkage on bottom). In both high and low resolution space, the points are coloured with respect to the value taken by the first diffusion coordinate in the low-resolution space. The lower right corner of the figure shows the scatter plot in which the first and second diffusion coordinates (DC) of the high-resolution space are plotted against the corresponding coordinate of the low-resolution space.

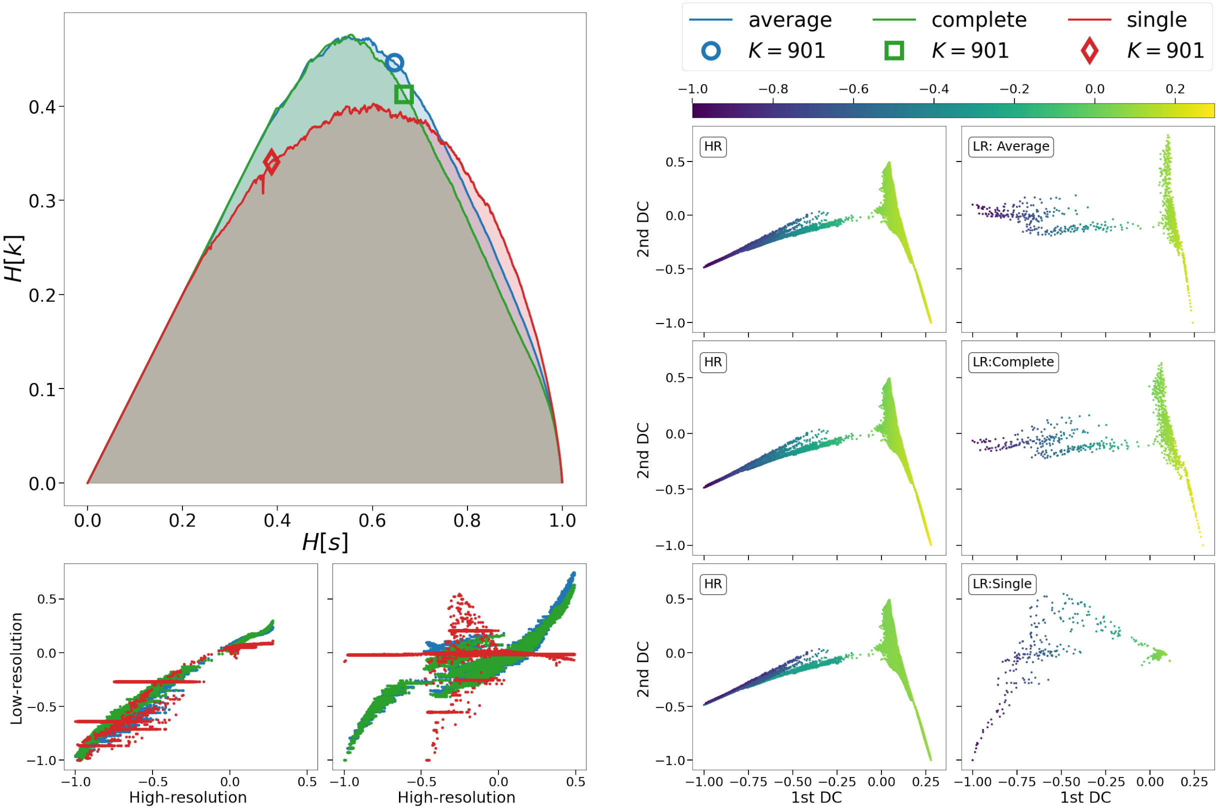


Figure 7: The panel aims to quantitatively and qualitatively compare the low-resolution representation (LR) of the configurational space explored by the humanised IgG4 monoclonal antibody during an MD simulation. These representations are obtained through three clustering protocol, for a number of clusters $K = 901$. The upper left-hand side of the figure shows the relevance-resolution curves obtained from clustering the MD trajectory, according to the average-linkage (blue), complete-linkage (green) and single-linkage (red) protocols. The system was analysed using a coarse representation in which only $C_\beta$ *atoms* are considered. The markers show where on the respective curve the low-resolution representations obtained by partitioning the system into a $K = 901$ clusters lie. On the right-hand side the graphs representing the points projected onto the space spanned by the first two diffusion coordinates. The graphs on the left show the diffusion space resulting from high-resolution representation (HR) where each point is a frame of the MD simulation and the distance between them is given by the RMSD calculated on the $C_\beta$ atoms. On the right the two-dimensional diffusion space resulting from the LR representation where each point is the centroid of a cluster and the distance between points is the linkage measure that produced the partition (average-linkage on top, complete-linkage in the middle and single-linkage on bottom). In both high and low resolution space, the points are coloured with respect to the value taken by the first diffusion coordinate in the low-resolution space. The lower right corner of the figure shows the scatter plot in which the first and second diffusion coordinates (DC) of the high-resolution space are plotted against the corresponding coordinate of the low-resolution space.
